# Supplementary material for: Predictive Event Segmentation and Representation with Neural Networks: A Self-Supervised Model Assessed by Psychological Experiments
Source: arXiv:2210.05710 source file (2022-10-04)
Supplement: Supplementary file 1 [file supplementary_material.tex]

\section{Supplementary Materials}

\textbf{Supplementary material for the dataset preparation:} Individual behaviors in the dataset are combined by a linear interpolation method. In order to preserve the natural continuity, behaviors are selected by keeping the distance between the end of the first and the start of the second behavior the smallest in all possible permutations.

With the aim of detecting whether those interpolation points affect the correlation score received by the computational models, we devised some control analyses. Results showed that the correlation scores of the computational models were still higher than the control models regardless of the quality of video (see Figure~\ref{fig:normal_model_segmentation_control_analyses} and Figure~\ref{fig:noisy_model_segmentation_control_analyses}).

\begin{figure}[h!]
\centering
  \includegraphics[width=\columnwidth]{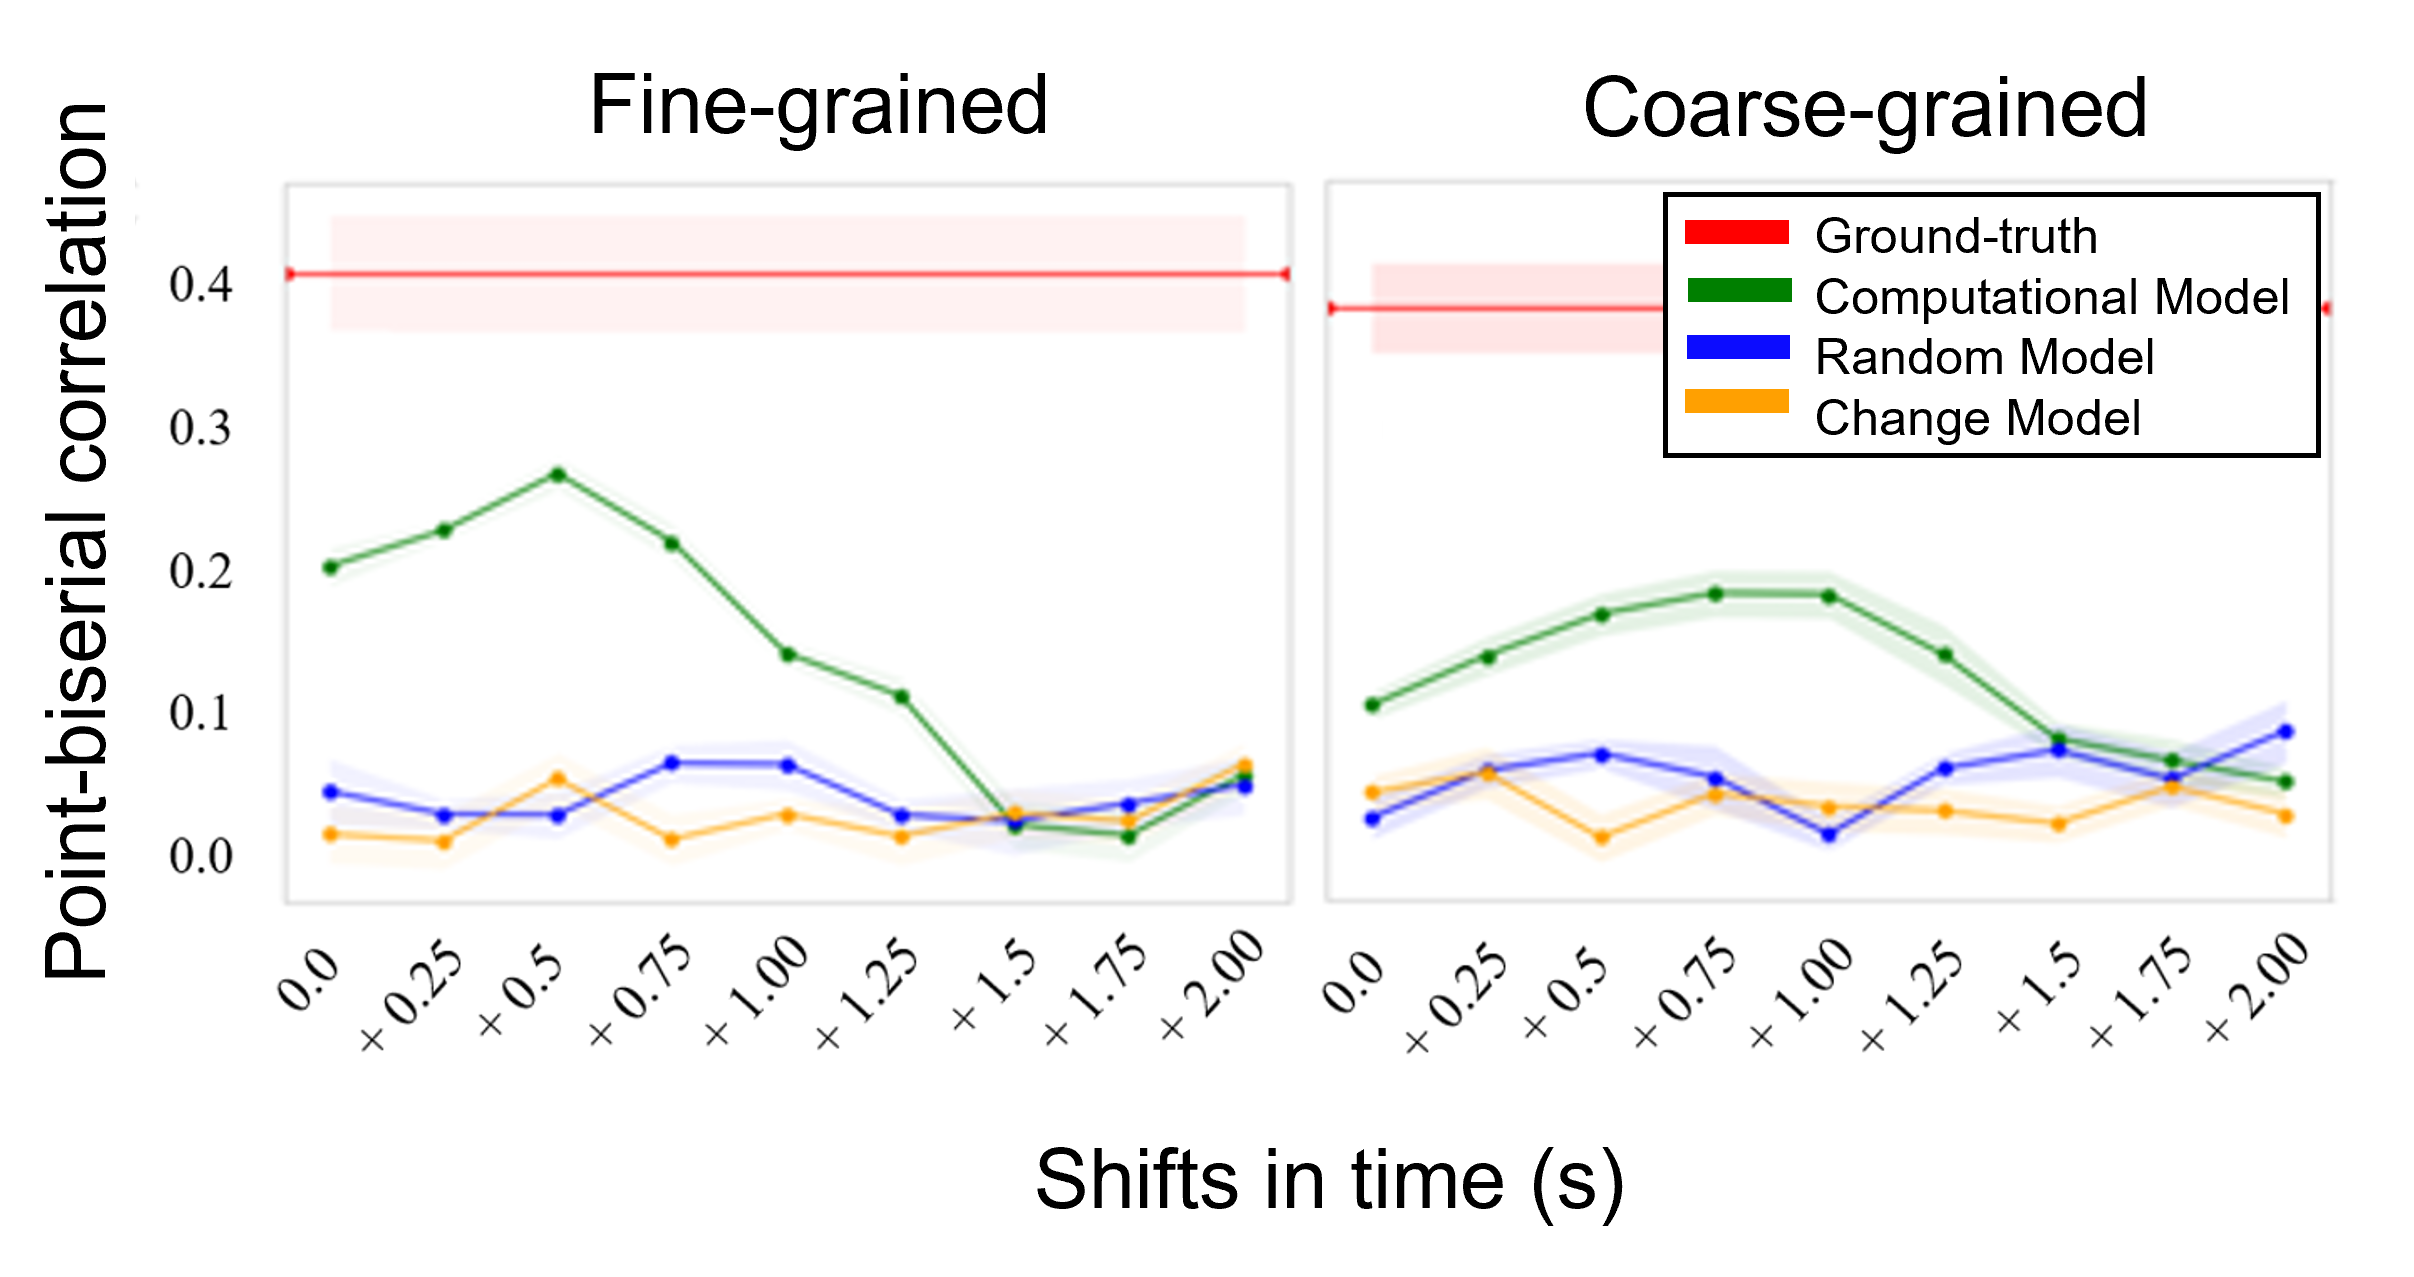}
    \caption{Time-dependent performances of the computational model for the normal video when the interpolation points were removed. Point-biserial correlations were calculated between the event boundary histograms as the ground-truth and the models’ event boundary decisions. Event boundary decisions of the models were shifted forward in time to reveal the time-dependent correlations. Performances of the model were not differed significantly for the fine- (r_{normal} = .199, r_{control} = .171, z = 0.335, p = .737, two-tailed) and coarse-grained segmentation (r_{normal} = .12, r_{control} = .06, z = 0.699, p = .484, two-tailed), when there was no time shift.}
\label{fig:normal_model_segmentation_control_analyses}
\end{figure}

\begin{figure}[h!]
\centering
  \includegraphics[width=\columnwidth]{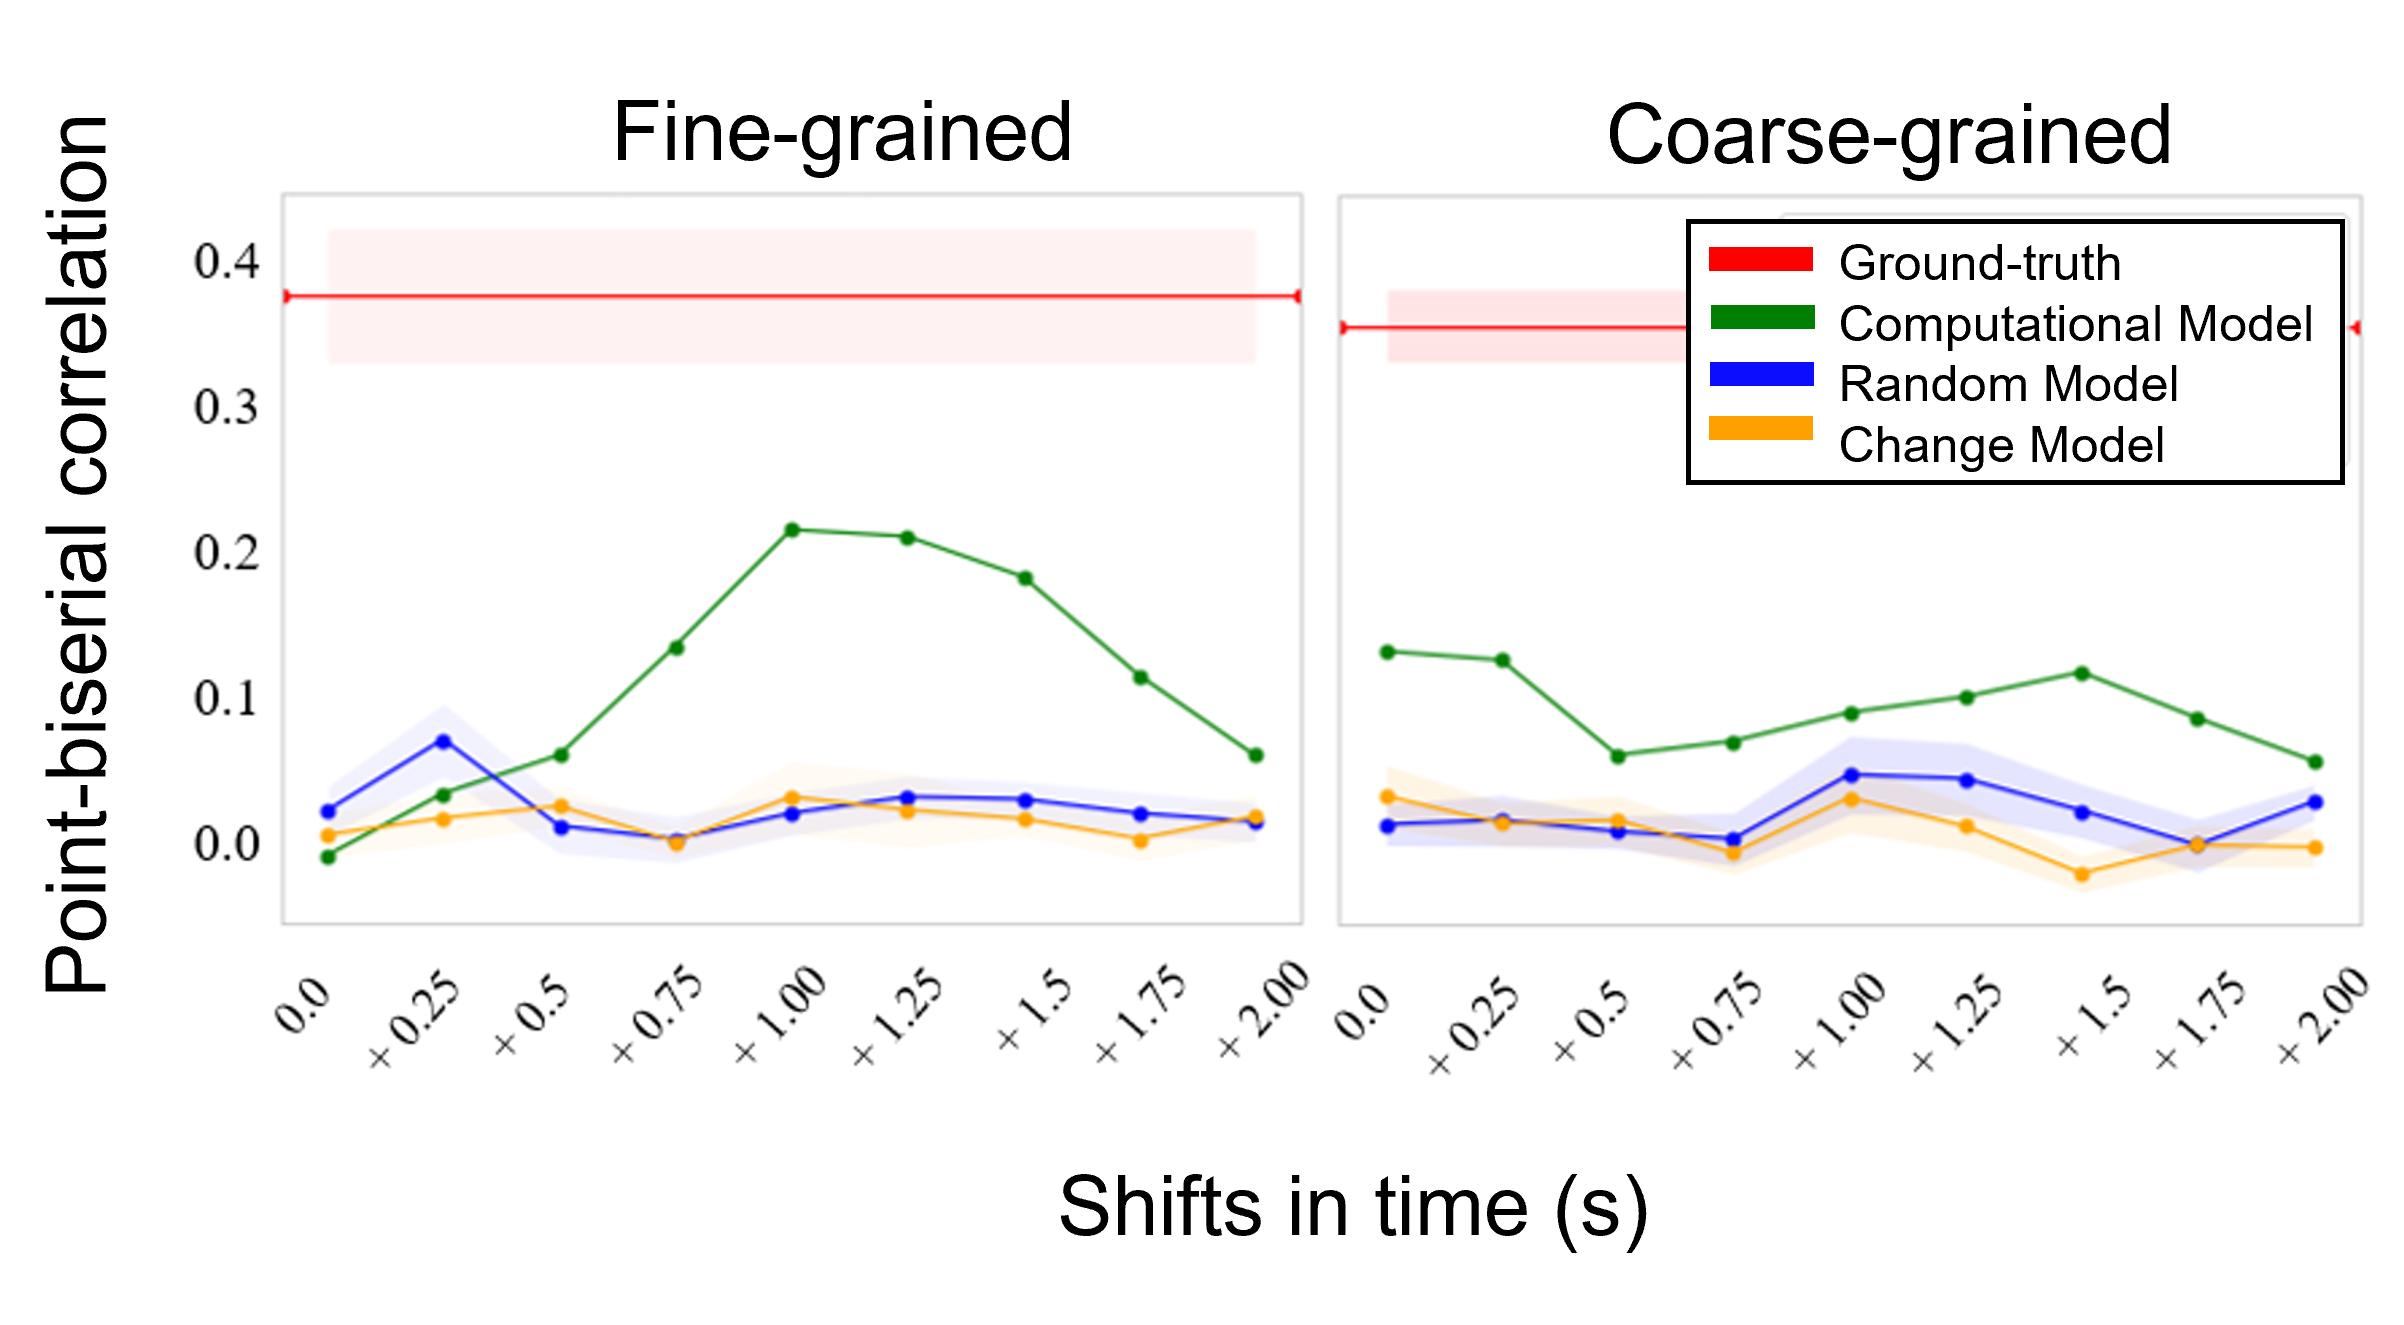}
    \caption{Time-dependent performances of the computational model for the noisy video when the interpolation points were removed. Point-biserial correlations were calculated between the boundary histograms as the ground-truth and the models’ boundary decisions shifted forward in time. Note that the hyperparameters of the model were not selected for the noisy video.}
\label{fig:noisy_model_segmentation_control_analyses}
\end{figure}

\textbf{Supplementary material for maintaining the data reliability:} With the aim of controlling the data reliability, a control behavior was added to the dataset, which occurs between 42.75-71.5 and 209.25-237.5. The control behavior is defined in the dataset as “lifting and lowering an object by hand,” which involves sharp hand movements in the Y dimension, appealing an event boundary response. Responses of the participants for the first and second observations were detected and turned into a mixture of Gaussian distributions. For the fine-grained segmentation, the normal distribution generated for each button pressing was determined to be N(t, 1), whereas, for the coarse-grained segmentation, it was determined to be N(t, 4) as the transition between two coarse-grained units might take more time than that of two fine-grained units. Then, the resulting distributions of each kind of observation are compared by the Pearson correlation coefficient. Responses of participants showing very weak or inverse (r < .1), but significant correlation (a = 0.05) were excluded. The data of three participants were excluded from the analysis by this technique.

\textbf{Supplementary material for the selection of hyperparameters:}

We determined the hyperparameters of the model for the fine-grained and the coarse-grained segmentation of the normal dataset/video; then, we re-used the same hyperparameters for the fine-grained and coarse-grained segmentation of the noisy video. Selected hyperparameters are given in Table~\ref{tab:hyperparameters}.

\begin{table}[h]
\centering
\caption{Hyperparameters of the Computational Model}
\label{tab:hyperparameters}
\begin{footnotesize}
\begin{tabular}{lll}
Parameters            & Fine-grained       & Coarse-grained       \\\hline
Event threshold       & 1.25               & 2.5                  \\\hline
Error window          & 10                 & 30                   \\\hline
Number of timesteps   & 5                  & 15                   \\\hline
Rehearsal             & 100                & 100                  \\\hline
Replay                & 2000               & 2000                 \\\hline
Number of epochs      & 10                 & 10                   \\\hline
Memory range          & 1                  & 1                    \\\hline
Activations functions & Relu               & Relu                 \\\hline
Optimizer             & ADAM               & ADAM                 \\\hline
Learning rate         & 0.0001             & 0.0001               \\\hline
Batch size            & 12                 & 12                   \\\hline
Hidden layers         & (256, 128, 64, 64) & (512, 256, 128, 128) \\\hline
\end{tabular}
\end{footnotesize}
\end{table}

\textbf{Supplementary material for the representation discovery techniques:}

\textbf{a) Estimated Event Representation in Computational Model (EER-CM):}

For calculating this metric, we developed a neural network classifier that takes PLD stream as input and predicts the corresponding event model id as output. In this way, the neural network classifier grasps the relationship between segmented events. Formally, the classifier $H$ does

\[H(S_{t-n:t})= M_t\]

That is, the classifier $H$ predicts the model $M$ at the time $t$ by receiving the sensory information $S$ with a window of $n$. After training $H$, representation $R_t$ for $S_t$ is received by feeding the model $S_{t-n:t}$. To find the similarity between two event segments, each sensory input $S_t$ is represented in a two-dimensional representational space by PCA (Principal Component Analysis) \citep{wold1987principal} or t-SNE (T-Distributed Stochastic Neighbor) \citep{van2008visualizing}. The representation $R_a$ for a given segment $S_{t1:t2}$ is found by 

\[\mu(R_{t1:t2})\]

From these representations, the similarity between two event segments is estimated by

\[Sim(S_{t1:t2},S_{t3:t4})= 1-Euclid(\mu(R_{t1:t2}), \mu(R_{t3:t4} ))\]

\textbf{b) Pairwise Event Distance in Computational Model (PED-CM)}

Recall that each event in our model is represented with a feed-forward neural network (FFNN). The pairwise distances between events are calculated by taking the distances between the outputs of the corresponding event models. The idea is, if two events are similar, then two event models trained for those events should also produce similar sequences of prediction. Thus, the similarity between those prediction sequences should indicate their relationships. For this technique, we compared two prediction sequences by a dynamic time warping method (DTW) \citep{Giorgino2009Computing}, which is a technique measuring the distance between two sequential data. Formally, suppose that $M_a$ predicts $S_{t1:t2}$ and $M_b$ predicts $S_{t3:t4}$, we computed the similarity between two segments by

\begin{multline*}
Sim(S_{t1:t2},S_{t3:t4}) = 
1 - DTW(M_a(S_{t1:t2}), M_b (S_{t1:t2} )) + \\
DTW(M_b (S_{t3:t4}), M_a (S_{t3:t4})) 
\end{multline*}

\textbf{Supplementary material for event sampling:} To sample from event segments, we computed the cumulative distance between each event and ordered them as a list. This resulted in two lists for fine-grained and coarse-grained events. From the ordered list of fine-grained events, we selected the top and bottom 5\% of all events; whereas from the ordered list of coarse-grained events, we selected the top and bottom 25\% of all events. We applied the same process for three techniques as they generated different distances between events (EER-CM/PCA, EER-CM/t-SNE, and PED-CM).
